# Supplementary material for: Fast, Exact Bootstrap Principal Component Analysis for p>1 million
Source: arXiv:1405.0922 source file (2014-05-14)
Supplement: Supplementary file 1 [file boot_pca_supplement_unblinded.pdf]

# Fast, Exact Bootstrap Principal Component Analysis for p> 1 million: Supplemental Matrials

Aaron Fisher, Brian Caffo, Brian Schwartz & Vadim Zipunnikov

May 13, 2014

## Contents

**1 Block matrix algebra for when the data cannot fit into memory 1**

**2 Random preconditioning for when the SVD fails to converge 2**

**3 Centering bootstrap samples by centering scores 3**

**4 Changing the sign of bootstrap PCs - dot product v. correlation 3**

**5 Supplemental figures for the EEG and MRI Datasets 4**

# 1 Block matrix algebra for when the data cannot fit into memory

When the number of measurements is especially large (i.e., $p$ >10,000), it is common that either the $p \times n$ data matrix $\mathbf{Y}$, or the $p \times B$ matrices storing each of the $K$ fitted PCs across bootstrap samples, may be too large to store in working memory. This issue can be remedied by using block matrix algebra to subdivide the SVD computation into a series of low memory steps.

The standard algorithm for calculating the SVD of a high dimensional $p \times n$ matrix $\mathbf{Y}$ begins by first calculating the $n \times n$ matrix $\mathbf{Y}'\mathbf{Y}$. Calculating the SVD of $\mathbf{Y}'\mathbf{Y}$ yields $\mathbf{UD}^2\mathbf{U}'$. The matrix $\mathbf{V}$ can then be calculated as $\mathbf{V} = \mathbf{YUD}^{-1}$. When $p$ is much larger than $n$, the computational complexity of this method is $O(pn^2)$.

For the case where $\mathbf{Y}$ is too large to be stored in working memory, define $\{s_1, s_2, ...s_m\}$ to be the set of $m$ indexing vectors, each of length $p/m$, such that the $p$-length concatenated vector $(s_1, s_2, ...s_m)$ is equal to vector $(1, 2, 3, ...p)$. Note that $\mathbf{Y}$ can now be partitioned as $\mathbf{Y}' = [\mathbf{Y}'_{[s_1,]}\ \mathbf{Y}'_{[s_2,]}\ ...\ \mathbf{Y}'_{[s_m,]}]$. The matrix

$\mathbf{Y}'\mathbf{Y}$ can be calculated as $\sum_{i=1}^{m} \mathbf{Y}'_{[s_i,]}\mathbf{Y}_{[s_i,]}$, where each term of the sum can be calculated separately. We can similarly partition $\mathbf{V}' = [\mathbf{V}'_{[s_1,]}\ \mathbf{V}'_{[s_2,]}\ ...\ \mathbf{V}'_{[s_m,]}]$, with $\mathbf{V}_{[s_m,]} = \mathbf{Y}_{[s_m,]}\mathbf{U}\mathbf{D}^{-1}$. Neither the entire matrix $\mathbf{Y}$ nor the entire matrix $\mathbf{V}$ need ever be stored in memory. (Zipunnikov et al., 2011)

For the bootstrap percentile intervals described in section 3.3.1 of the main paper, note that the bootstrap CIs for each block of $\mathbf{V}$ can be calculated separately. In each bootstrap sample, the fitted PCs can be partitioned as

$$\mathbf{V}^{b'}_{[,1:K]} = [\mathbf{V}^{b'}_{[s_1,1:K]}\ \mathbf{V}^{b'}_{[s_2,1:K]}\ \cdots\ \mathbf{V}^{b'}_{[s_m,1:K]}]$$

and calculated according to the relation $\mathbf{V}^{b}_{[s_i,1:K]} = \mathbf{V}_{[s_i,]}A^{b}_{[,1:K]}$. The bootstrap percentiles for the elements of each partition of the PC matrix can be calculated separately, without storing the high dimensional the bootstrap distribution of $\mathbf{V}^{b}_{[,1:K]}$ in working memory. Of the different CIs and CRs proposed in section 3.3 of the main paper, percentile intervals form the only case where memory constraints become a potential issue in the bootstrap calculations. For the moment-based pointwise intervals, as well as the other confidence regions discussed in section 3.3, only the low dimensional bootstrap distribution of $A^{b}_{[,1:K]}$ is required.

# 2 Random preconditioning for when the SVD fails to converge

We find in approximately 4% of bootstrap samples from the MRI dataset, that although a solution to the SVD of $\mathbf{D}\mathbf{U}'\mathbf{P}^b$ exists, the SVD function fails to converge. We handle these cases by randomly preconditioning the matrix $\mathbf{D}\mathbf{U}'\mathbf{P}^b$, and reapplying the SVD function. We then adjust the output of this preconditioned SVD operation to find the solution for the SVD of the original matrix $\mathbf{D}\mathbf{U}'\mathbf{P}^b$.

The specific steps of this adjusted SVD algorithm are described below, in terms of their application to an arbitrary $n \times m$ matrix $\mathbf{\Sigma}$.

- Step 1: To find $svd(\mathbf{\Sigma})$, first generate a two random orthonormal matrices $\mathbf{Q}_n$ and $\mathbf{Q}_m$, of dimension $n \times n$ and $m \times m$ respectively. Each matrix can be obtained by taking the QR decomposition of a square matrix of random normal noise.
- Step 2: Calculate the SVD of $\mathbf{Q}'_n\mathbf{\Sigma}\mathbf{Q}_m$, and denote the result as $\mathbf{V}\mathbf{D}\mathbf{U}'$.
- Step 3: If this SVD operation also fails to converge, repeat steps 1-2 until either a solution is found, or a pre-specified maximum number of attempts is reached. We generally find that a single iteration is sufficient.
- Step 4: Write the SVD of $\mathbf{\Sigma}$ as $(\mathbf{Q}_n\mathbf{V})\mathbf{D}(\mathbf{Q}_m\mathbf{U})'$.

Note $(\mathbf{Q}_n\mathbf{V})$ and $(\mathbf{Q}_m\mathbf{U})$ are both orthonormal, $\mathbf{D}$ is diagonal, and

$$(\mathbf{Q}_n\mathbf{V})\mathbf{D}(\mathbf{Q}_m\mathbf{U})' = \mathbf{Q}_n\mathbf{V}\mathbf{D}\mathbf{U}'\mathbf{Q}'_m = \mathbf{Q}_n\mathbf{Q}'_n\mathbf{\Sigma}\mathbf{Q}_m\mathbf{Q}'_m = \mathbf{\Sigma}$$

So $(\mathbf{Q}_n\mathbf{V})\mathbf{D}(\mathbf{Q}_m\mathbf{U})'$ is indeed a solution to the SVD of $\mathbf{\Sigma}$. If the SVD of $\mathbf{\Sigma}$ is unique, then $(\mathbf{Q}_n\mathbf{V})\mathbf{D}(\mathbf{Q}_m\mathbf{U})'$ is the unique solution to the SVD.

When $\mathbf{\Sigma}$ is a square matrix, this procedure can be simplified by letting $\mathbf{Q}_m = \mathbf{Q}_n$. The procedure can also be made slightly faster by replacing $\mathbf{Q}_m$ and $\mathbf{Q}_n$ with random permutation matrices.

# 3 Centering bootstrap samples by centering scores

Centering the $p \times n$ matrix $\mathbf{Y}$ can be achieved by right multiplying by $(\mathbf{I}_n - (1/n)\mathbf{1}_n\mathbf{1}_n')$, where $\mathbf{I}_n$ is the $n \times n$ identity matrix, and $\mathbf{1}_n$ is the $n$-length vector of ones. Since $\mathbf{Y}(\mathbf{I}_n - (1/n)\mathbf{1}_n\mathbf{1}_n') = \mathbf{VDU}'(\mathbf{I}_n - (1/n)\mathbf{1}_n\mathbf{1}_n')$, centering $\mathbf{Y}$ is equivalent to centering the $n \times n$ matrix of scores, $\mathbf{DU}'$.

Similarly, consider the bootstrap sample $\mathbf{Y}^b = \mathbf{YP}^b$. Because $\mathbf{YP}^b(\mathbf{I}_n - (1/n)\mathbf{1}_n\mathbf{1}_n') = \mathbf{VDU}'\mathbf{P}^b(\mathbf{I}_n - (1/n)\mathbf{1}_n\mathbf{1}_n')$, centering $\mathbf{Y}^b$ is equivalent to centering the $n \times n$ matrix of resampled scores, $\mathbf{DU}'\mathbf{P}^b$. Instead of taking the SVD of the resampled scores, we can simply take the SVD of the resampled *and centered* scores.

# 4 Changing the sign of bootstrap PCs - dot product v. correlation

Because the bootstrap principal components (PCs) are only unique to sign, and sign does not affect our interpretation of the PCs, it can be useful to match the sign of all bootstrap PCs before calculating their variability. Let $\mathbf{v}$ denote a $p$-length fitted PC vector in the original sample, and $\mathbf{v}^b$ be the corresponding fitted PC in the $b^{th}$ bootstrap sample. It has generally been proposed that each $\mathbf{v}^b$ be adjusted to match the sign of $\mathbf{v}$. Some have proposed matching by switching the sign of $\mathbf{v}^b$ whenever the arithmetic correlation between between $\mathbf{v}$ and $\mathbf{v}^b$ is negative (Jackson, 1995; Babamoradi et al., 2012). Others have proposed methods equivalent to changing the sign of $\mathbf{v}^b$ when the dot product $\mathbf{v}'\mathbf{v}^b$ is negative (Lambert et al., 1991; Milan and Whittaker, 1995). In this section, we compare cases there these two methods disagree, and argue that the results of the dot product approach are more interpretable.

Clearly these two methods are related, as $cov(\mathbf{v}, \mathbf{v}^b) = (\mathbf{v}'\mathbf{v}^b - \mu\mu^b p)/(p-1)$, where $\mu$ and $\mu^b$ are the arithmetic means of $\mathbf{v}$ and $\mathbf{v}^b$ respectively. We use the term "arithmetic" to emphasize the fact that while $\mu = \frac{1}{p}\sum_{j=1}^{p}\mathbf{v}_{[j]}$, the elements of $\mathbf{v}$ do not form a random sample, and $\mu$ is not a sample mean. Although the two methods for changing the sign of $\mathbf{v}^b$ will general produce the same result, they may disagree when $\mu$ is far from zero, such as when $\mathbf{v}$ represents a flat mean shift.

Figure 1 shows example of when the two methods give different results. In the left panel, $cor(\mathbf{v}, \mathbf{v}^b) = -1$, but $\mathbf{v}'\mathbf{v}^b = .9$. Here, the correlation rule would suggest that the sign of $\mathbf{v}^b$ be inverted, but the dot product rule would imply that the sign should not be inverted. The right panel gives the opposite case,

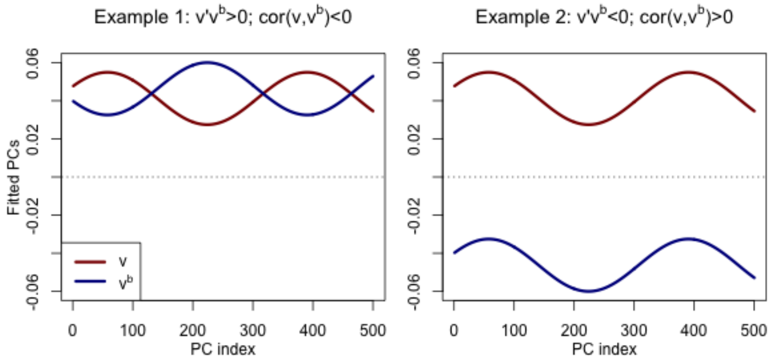


Figure 1: Comparison of axis reflections methods - Consider the case when the sample principal component, denoted as $\mathbf{v}$, roughly corresponds to a mean shift. The left panel shows a case where the bootstrap estimate of $\mathbf{v}$, denoted as $\mathbf{v}^b$, is negatively correlated with $\mathbf{v}$, but where $\mathbf{v}'\mathbf{v}^b > 0$. The right panel shows a case where the $\mathbf{v}$ and $\mathbf{v}_0$ are positively correlated, but $\mathbf{v}'\mathbf{v}^b < 0$. We argue that a reflection should be applied for the case shown on the right, but not for the case shown on the left.

where the dot product rule would imply that the sign of $\mathbf{v}^b$ be switched, but the correlation rule implies that it should not be. In both examples, we find the results of the dot product rule to be more intuitive. For PCs that are fairly flat, the correlation rule has the potential to create bimodal bootstrap distributions of $\mathbf{v}^b$ on either side of the zero line. This results in confidence intervals that include zero, and are not centered around the sample PC $\mathbf{v}$.

# 5 Supplemental figures for the EEG and MRI Datasets

Figure 2 shows approximate reconstructions of the observed subjects' EEG measurements using only the $K$ leading PCs, for $K = 1, 2, 5$, and 391. We see that the more PCs are included in the approximation, the more variability is retained from the original dataset. In the first panel ($K = 1$), the variability in the reconstructed dataset is roughly due to different within-subject average $NP_\delta$ levels. This panel also shows the average $NP_\delta$ across subjects, denoted by $\boldsymbol{\mu}$. In panel 2 we add in variability attributable to the second PC ($K = 2$), and see that reconstructed $NP_\delta$ measurements now also vary in terms of broad oscillatory patterns in the early stages of sleep. Panel 3 shows variability due to the first five PCs ($K = 5$), and highlights how the primary patterns in $NP_\delta$ variability take place in the first three hours of the night. The final plot shows the full reconstruction of the dataset with all $n - 1$ PCs, and contains the most

overall variability.

Figure 3 shows the cumulative variance explained by the first 30 PCs of the EEG dataset, and by the first 30 PCs of the MRI dataset. These curves are proportional to the cumulative sum of the eigenvalues of the sample covariance matrices for each dataset.

# References


Babamoradi, H., van den Berg, F., and Rinnan, Å. (2012). Bootstrap based confidence limits in principal component analysis–a case study. *Chemometrics and Intelligent Laboratory Systems*.

Jackson, D. A. (1995). Bootstrapped principal components analysis- reply to mehlman et al. *Ecology*, 76(2):644–645.

Lambert, Z. V., Wildt, A. R., and Durand, R. M. (1991). Approximating confidence intervals for factor loadings. *Multivariate Behavioral Research*, 26(3):421–434.

Milan, L. and Whittaker, J. (1995). Application of the parametric bootstrap to models that incorporate a singular value decomposition. *Applied Statistics*, pages 31–49.

Zipunnikov, V., Caffo, B., Yousem, D. M., Davatzikos, C., Schwartz, B. S., and Crainiceanu, C. (2011). Functional principal component model for high-dimensional brain imaging. *NeuroImage*, 58(3):772–784.

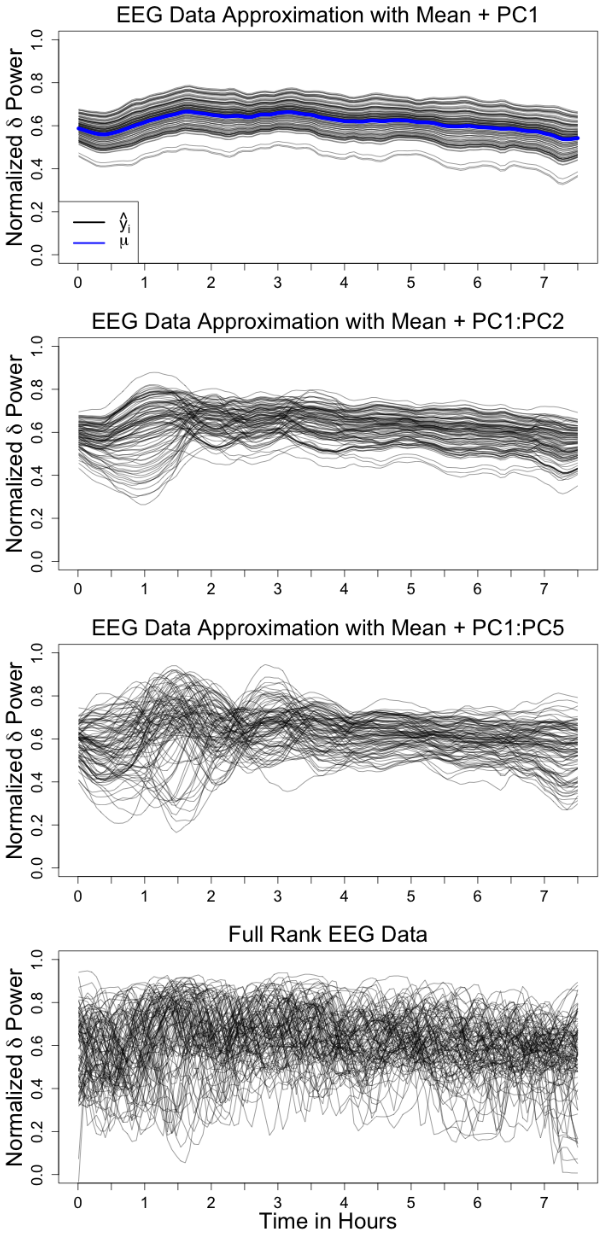


Figure 2: Reconstructions of EEG data with leading PCs - The first three panels respectively show approximations constructed using the first PC, the first two PCs, and the first five PCs. The first panel also shows the mean $NP_\delta$ across subjects, denoted by $\boldsymbol{\mu}$. The bottom panel uses all of the PCs to reconstruct the sample points exactly. To avoid over-plotting, reconstructions are shown only for a random subsample of 100 subjects.

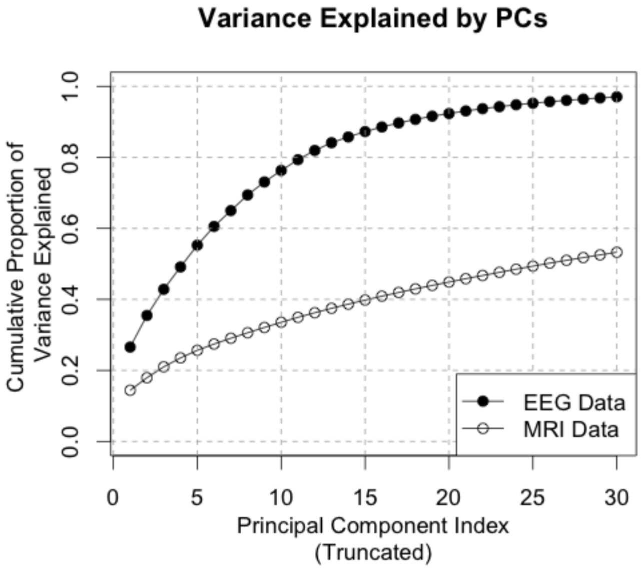


Figure 3: Cumulative proportion of variance explained by the first 30 PCs.
